# Supplementary material for: Decentralized utility- and locality-aware replication for heterogeneous DHT-based P2P cloud storage systems
Source: arXiv:1907.11997 source file (2019-07-28)
Supplement: Supplementary file 1 [file Appendix.tex]

\newpage
\appendix
\section{Additional performance graphs}
\label{pyramid:sec_appendix}
%%%%%%%%%%%%%%%%%%%%%%%%%%%%%%%%%%%%%%%%%%%%%%%%%%%%%%%

\begin{figure}
\centering
\centering
    \scalebox{0.7}{\input{Graphs/availability.tex}}
    \caption{}
    \label{fig:avelatency}
\end{figure}

\begin{figure}
\centering
\centering
    \scalebox{0.7}{\input{Graphs/pure-availability.tex}}
    \caption{}
    \label{fig:avelatency}
\end{figure}

\begin{figure}
\centering
\centering
    \scalebox{0.7}{\input{Graphs/scalability.tex}}
    \caption{}
    \label{fig:avelatency}
\end{figure}
